# Supplementary material for: The Role of Bases in Quantum Optimal Control
Source: arXiv:2405.20889 source file (2024-08-06)
Supplement: Supplementary file 1 [file role_of_QOC_supps.pdf]

# Supplemental Material – The Role of Bases in Quantum Optimal Control

Alice Pagano,[1,2,3] Matthias M Müller,[4] Tommaso Calarco,[4,5,6] Simone Montangero,[1,2,3] and Phila Rembold[2,5,7]

[1]*Institute for Complex Quantum Systems, Ulm University, Albert-Einstein-Allee 11, 89069 Ulm, Germany*

[2]*Dipartimento di Fisica e Astronomia "G. Galilei" & Padua Quantum Technologies Research Center, Università degli Studi di Padova, 35131 Padova, Italy*

[3]*INFN, Sezione di Padova, via Marzolo 8, 35131 Padova, Italy*

[4]*Peter Grünberg Institute – Quantum Control (PGI-8), Forschungszentrum Jülich GmbH, 52425 Jülich, Germany*

[5]*Institute for Theoretical Physics, University of Cologne, 50937 Köln, Germany*

[6]*Dipartimento di Fisica e Astronomia, Università di Bologna, 40127 Bologna, Italy*

[7]*Atominstitut, Technische Universität Wien, Stadionallee 2, 1020 Wien, Austria*

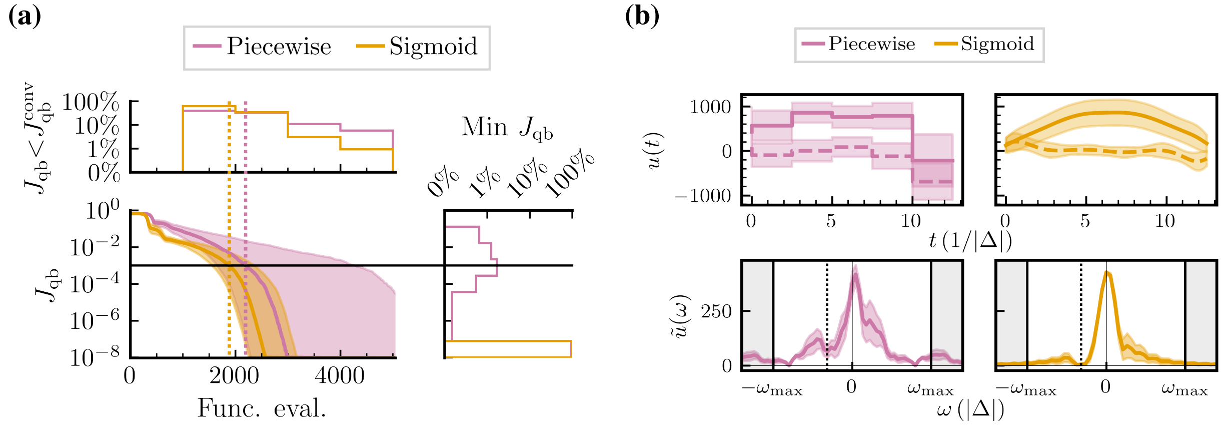


Figure 1: **(a)** Comparison between sigmoid and piecewise basis for qutrit problem. The convergence probability for the piecewise is $P_c = 97.6\%$, the one for the sigmoid is $P_c = 99.96\%$ as reported in the main text. The number of parameters optimized is $N_c = 6$. **(b)** Pulse and spectrum comparison.

## I. THE PIECEWISE-CONSTANT BASIS

Many algorithms commonly apply the piece-wise constant basis. Their most prominent representatives are GRAPE [1] and Krotov's method [2], both of which are gradient-based open-loop optimisation methods. The sigmoid basis represents the same function-space as the piece-wise constant basis, if the sigmoid width is $\sigma \ll 1$ creating genuine step functions. In general, all basis elements are considered to be of the same length for the piecewise-constant basis which is taken into consideration by

$$\tau_p = \tau_0 + p\Delta\tau, \text{ where } \Delta\tau = \frac{\tau_N - \tau_0}{N}. \tag{1}$$

The parameter scaling the $p^{\text{th}}$ sigmoid basis element is given by $A_p$. Similarly, the $k^{\text{th}}$ piece-wise constant element is scaled by $u^{(k)}$ in analogy to GRAPE, where $u^{(0)} = u^{(N+1)} = 0$. Assuming that $\sigma \ll \Delta\tau$, they are connected by the following relationships:

$$\begin{aligned} A_p &= u^{(p+1)} - u^{(p)}, \\ u^{(k)} &= \sum_{p=0}^{k-1} A_p. \end{aligned} \tag{2}$$

To see how this transformation may be exploited in a gradient-based context, please refer to Ref. [3]. The example problem presented in Sec. IIIB is known to be well optimisable using the piecewise-constant basis [4]. To show that the sigmoid basis is not only in principle equivalent but also a sensible replacement, we compare the two bases in Fig. 1 for the NOT gate optimization.

## II. HYPERPARAMETERS

The selected hyperparameters for the test problems in Sec. III are representative and aim to yield the best average results for convergence probability. To demonstrate this, in the following we show that varying the hyperparameters does not alter the results.

In Fig. 2, the convergence traces for a different set of hyperparameters for different number of qubits are reported. The parameters are assumed to be the one fixed in Table I unless stated differently on top of the plot. In more detail, we present the results for two qubits with varying final times $T$, for three qubits with different numbers of optimization parameters $N_{\text{opt}}$ and for four qubits with different maximum frequencies $\omega_{\max}$. By examining the results, as summarized in Table I, we confirm that for this problem, the sinc basis converges faster than the Fourier basis, and the sigmoid basis does not perform well.

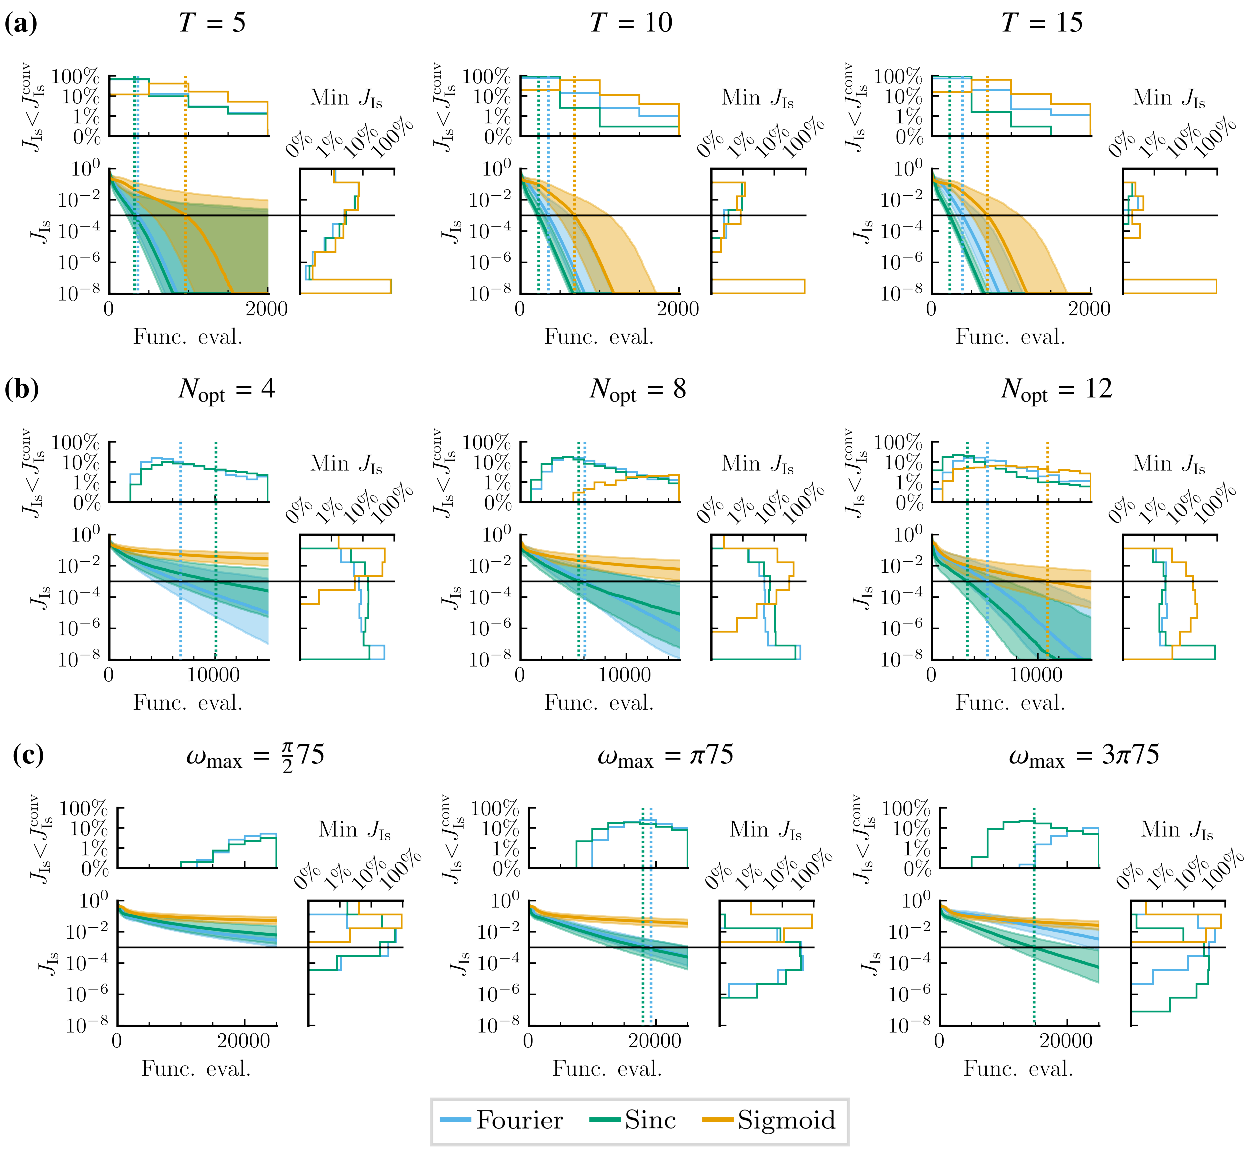


Figure 2: Comparing convergence traces with varying hyperparameters. (a) 2-qubit analysis involves changes in the final time $T$ (b) 3-qubit analysis focuses on variations in optimization parameters $N_{\text{opt}}$ (c) 4-qubit analysis explores variations in the maximum frequency $\omega_{\max}$.

For the single qubit gate problem, we compare the histogram in Fig. 3 showing the percentage of optimizations that have converged below different thresholds as a function of the number of iterations, particularly for $J_{\text{qb}}^{\text{conv}} = \{10^{-6}, 10^{-4}, 10^{-2}\}$. The quicker convergence rate of the sigmoid basis method remains consistent across all thresholds.

| $N$ | | 2 | | | 3 | | | 4 | | |
|---|---|---|---|---|---|---|---|---|---|---|
| $T$ | | 5 | 10 | 15 | | 20 | | | 75 | |
| $\omega_{\max}$ | | | $2\pi 20$ | | | $2\pi 20$ | | $\frac{\pi}{2}75$ | $\pi 75$ | $3\pi 75$ |
| $N_{\text{opt}}$ | | | 12 | | 4 | 8 | 12 | | 16 | |
| Fourier | $P_c$ | **84.85%** | **97.85%** | **99.45%** | **89.5%** | **93.2%** | **95.85%** | **12.5%** | **83.05%** | **22.45%** |
| | $\nu_c$ | 362 | 351 | 386 | 6749 | 6084 | 5234 | – | 19219 | – |
| sinc | $P_c$ | **83.85%** | **98.05%** | **99.5%** | **78.5%** | **91.05%** | **96.25%** | **7.95%** | **81.6%** | **89.6%** |
| | $\nu_c$ | 316 | 230 | 225 | 10086 | 5509 | 3338 | – | 17964 | 14794 |
| sigmoid | $P_c$ | **82.9%** | **97.85%** | **99.2%** | **1.85%** | **32.0%** | **79.7%** | **0%** | **0%** | **0%** |
| | $\nu_c$ | 963 | 681 | 700 | – | – | 10939 | – | – | – |

Table I: For 2, 3, and 4 qubits, the hyperparameters are associated with convergence probabilities $P_c$ and convergence periods $\nu_c$ for the three bases tested.

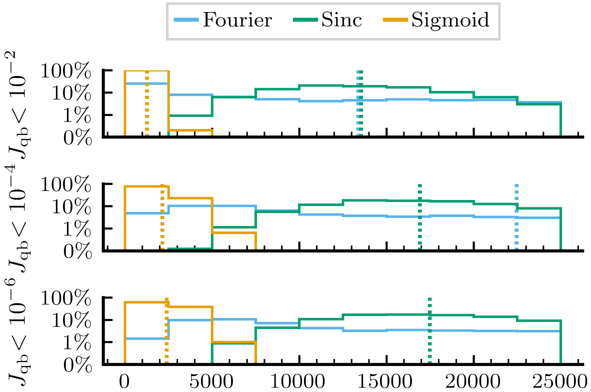


Figure 3: Comparison of the histograms representing the percentage of optimizations that have reached various cutoff thresholds ($J_{\text{qb}}^{\text{conv}}$) for the single qubit gate problem.

## III. AUTOMATIC DIFFERENTIATION

To show that our analysis is independent of the optimisation method, we confirm the results from the Ising chain with an AD-based optimisation. AD allows the calculation of gradients directly from the code [5, 6]. The optimisation was implemented using the JAX library [7] in python and hyperparameters specified in Table II. The number of parameters was chosen to be

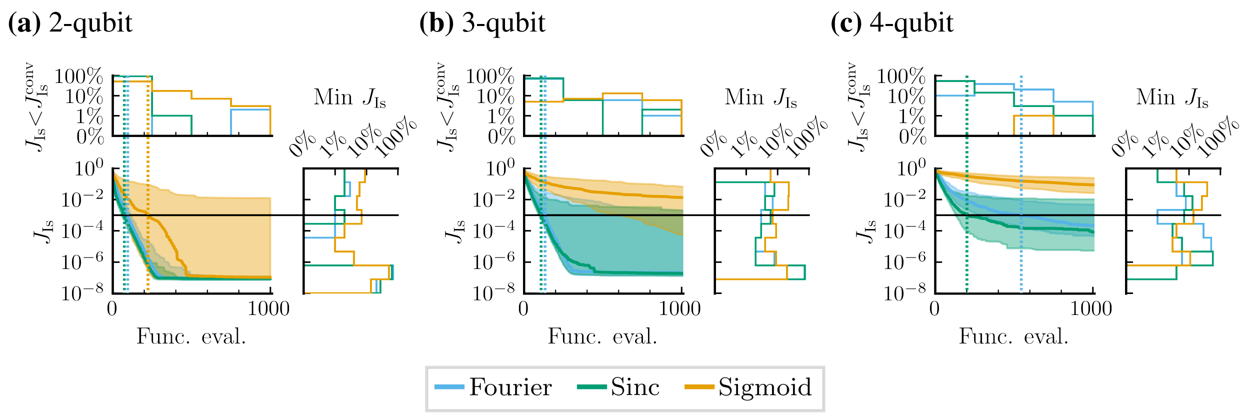


Figure 4: Ising chain convergence traces with AD for 100 different optimisations for 2, 3, and 4 qubits respectively. The main plot show the median convergence trace. The black horizontal line represents the threshold at $10^{-3}$. The histogram above is the percentage of optimisations that have dropped below the threshold within the number of iterations. Similarly, the histogram on the right show the final value of the cost function. All optimisations were stopped at $10^{-7}$.

twice as high for the sigmoid basis as it provides better convergence and is feasible with the applied gradient-based updating algorithm ADAM [8]. In this framework, we optimise the parameters as well as the superparameters to make a point of not using dCRAB. This is possible as ADAM imposes fewer restrictions on the number of parameters.

The results in Fig. 4 show that the Fourier and sinc bases outperform the sigmoid basis, even though the ladder is provided with a higher number of parameters. The results confirm the speedup in convergence of the sinc basis, especially in the case of four qubits as summarized in Table II. The optimisation is repeated 100 times.

## IV. SIGMOID BASIS

We consider the pulse basis elements $f(t)$ to be sigmoid functions. Sigmoids can in general be defined as the integral of a function with a single maximum at the centre. For the sake of simplicity, we only consider the sigmoid function that is defined by the integral of a Gaussian defined as

$$\begin{aligned} f(t) &= \frac{A_p}{\sqrt{2\pi}\sigma} \int_{-\infty}^{t} e^{-\frac{1}{2}\left(\frac{t'-\tau_p}{\sigma}\right)^2} dt' \\ &= \frac{A_p}{2}\left(1 + \operatorname{erf}\left(\frac{t-\tau_p}{\sqrt{2}\sigma}\right)\right). \end{aligned} \tag{3}$$

| | | $N$ | 2 | 3 | 4 |
|---|---|---|---|---|---|
| | | $T$ | 15 | 20 | 75 |
| | | $\omega_{\text{max}}$ | $2\pi$ | $2\pi$ | $4\pi$ |
| Fourier | | $N_{\text{opt}}$ | 24 | 30 | 30 |
| | | $P_c$ | **94.0%** | **87.0%** | **86.0%** |
| | | $\nu_c$ | 95 | 133 | 546 |
| sinc | | $N_{\text{opt}}$ | 24 | 30 | 30 |
| | | $P_c$ | **95.0%** | **86.0%** | **76.0%** |
| | | $\nu_c$ | 74 | 108 | 201 |
| sigmoid | | $N_{\text{opt}}$ | 48 | 60 | 60 |
| | | $P_c$ | **78.0%** | **45.0%** | **24.0%** |
| | | $\nu_c$ | 224 | – | – |

Table II: Ising chain optimisation performed with AD for 2, 3, and 4 qubits. The hyperparameters were empirically chosen to improve the convergence period. They are displayed together with the convergence probability $P_c$, and convergence period $\nu_c$ for the three tested bases.

Each element is characterised by the amplitude $A_p$ of the Gaussian, the centre time $\tau_p$ and the width $\sigma$. Accordingly, the sigmoid function resembles a smooth step function going from 0 to $A_p$ at a time $\tau_p$. Restrictions on the first derivative and hence rise time and bandwidth can be enforced via $\sigma$. As an example, to limit the gradient to that of a linear ramp of length $t_{\text{rise}}$ from 0 to $A_{\text{max}}$ one should set $\sigma \geq \sqrt{2/\pi}\ t_{\text{rise}}$. The difference made by the choice of $\sigma$ is illustrated in Fig. 5. Similarly, we can restrict the pulse length and amplitude via $A_p$ and $\tau_p$ as discussed in Ref. [3].

The sigmoid basis is composed of spectrally narrow elements with a time-limited derivative. As a result its bandwidth envelope is predictable. The spectrum of a pulse $u(t)$ constructed from a time-limited sum of $N$ sigmoid elements reads

$$\mathcal{F}[u(t)] = \frac{1}{i\omega} e^{-\frac{1}{2}\sigma^2\omega^2} \sum_{p=0}^{N} A_p e^{i\tau_p\omega}. \tag{4}$$

From this expression, one can derive a bandwidth envelope for any constructible pulse, which is only dependent on $\sigma$, $A_{\text{max}}$, the first rise time $\tau_0$, and the maximal rise time $\tau_N$. To do so, we consider the pulse with the highest possible integral, i.e. a square pulse with amplitude $A_{\text{max}}$. As the integral corresponds to the zero-frequency component of the spectrum and the pulse is

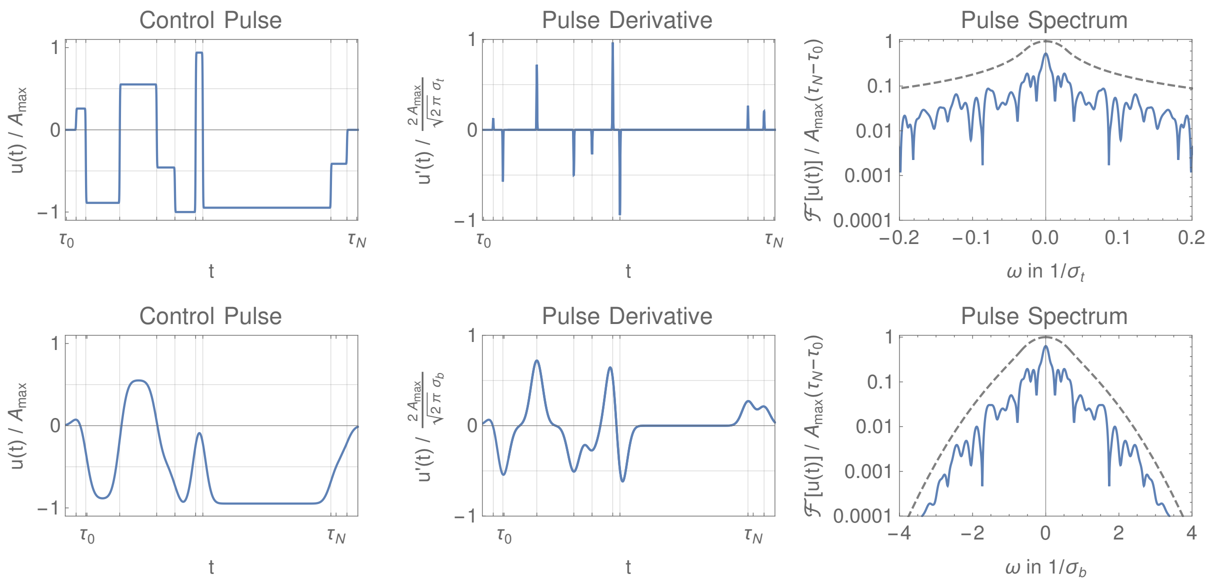


Figure 5: The effect of $\sigma$. From left to right, one can see apulse composed via the sigmoid basis, its derivative, and its spectrum. The top row shows a pulse constructed using a small width $\sigma_t = \frac{1}{20}\sigma_b$ while the bottom is made up of elements with $\sigma_b$. Please note that the right column is plotted over the same frequency range. The dashed line shows the respective bandwidth envelope. This figure was taken from Ref [3] with the author's permission.

symmetric, we can deduce the amplitude of the bandwidth limiting envelope $Y^{\infty}_{\max}$ shown in Fig. 6,

$$Y^{\infty}_{\max}(\omega) = A_{\max}(\tau_N - \tau_0)\, e^{-\frac{1}{2}\sigma^2\omega^2}. \tag{5}$$

This relation holds for infinitely many basis elements. However, the limit for a pulse constructed from $N$ basis elements is given by

$$k = \frac{(\tau_N - \tau_0)\omega}{2N},$$
$$Y^{N}_{\max} = Y^{\infty}_{\max} \begin{cases} -1/k & k \le -\frac{\pi}{2} \\ \sin k/k & -\frac{\pi}{2} < k < \frac{\pi}{2} \\ +1/k & k \ge \frac{\pi}{2} \end{cases}. \tag{6}$$

The center part sinc($k$) represents the Fourier transform of a square pulse of length $(\tau_N - \tau_0)/N$. The bandwidth envelope $Y^{N}_{\max}$ is shown for different values of $N$ in Fig. 6.

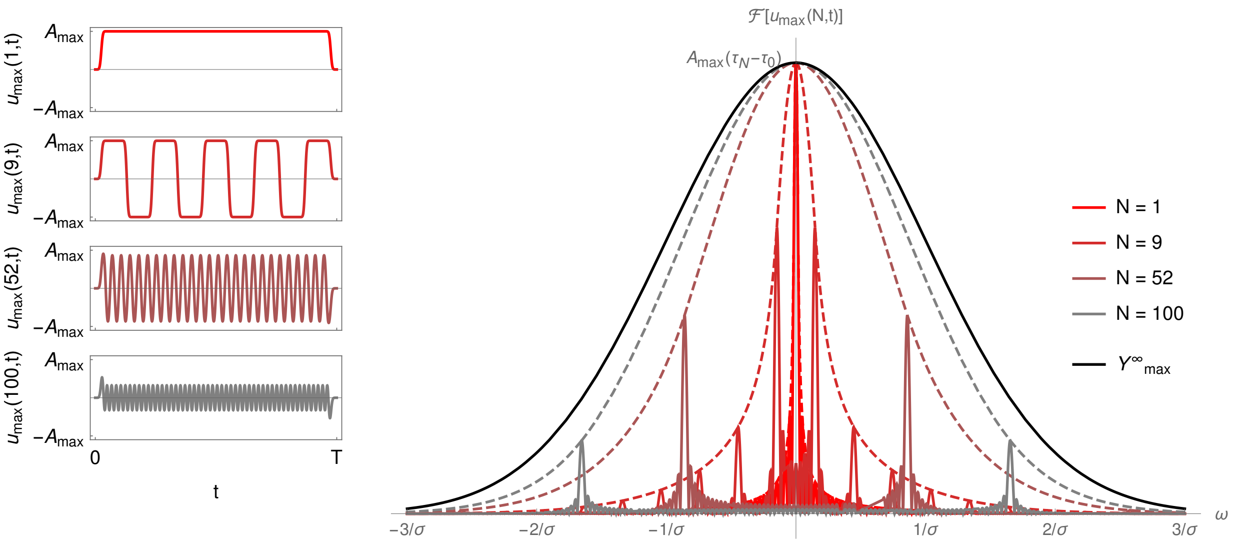


Figure 6: Control pulses composed to be time- and amplitude-limited and their corresponding spectra. The dashed lines represent $Y^N_{\max}$, the solid line gives $Y^\infty_{\max}$. This figure was taken from Ref [3] with the author's permission.

## V. SIGMOID IN DRAG

In zeroth order, DRAG creates pulses which methodically avoid unwanted transitions at a frequency $\Delta_0$. Here, we suggest a way to directly implement that condition in the pulses during optimisation. Please note that the following Appendix directly follows Ref. [3].

A complex pulse $u(t) = I(t) + iQ(t)$ has an asymmetric spectrum. By exploiting the relationship between the in-phase I-component $I(t)$ and quadrature Q-component $Q(t)$, specific components can be set to zero. First, let us consider a real function $f(t)$ which is limited in time i.e. $f(0) = f(T) = 0$. Its Fourier transform is given by $\mathcal{F}[f(t)] = Y(\omega)$. The Fourier identity for the spectrum of the function's first derivative reads:

$$\begin{aligned}\mathcal{F}[f'(t)] = X(\omega) = -i\omega Y(\omega)\\ 0 = Y(\omega) + i\frac{X(\omega)}{\omega}.\end{aligned} \tag{7}$$

To ensure that the spectrum of the complex pulse $u(t)$ has a node at $\Delta_0$, we can define the pulse components as

$$\begin{aligned}I(t) &= f(t) \text{ and}\\ Q(t) &= -\frac{f'(t)}{\Delta_0},\end{aligned} \tag{8}$$

making its Fourier transform

$$\begin{aligned}\mathcal{F}[u(t)] &= \mathcal{F}[I(t)] + \mathcal{F}[iQ(t)] \\ &= \mathcal{F}[f(t)] - i\mathcal{F}\left[-\frac{f'(t)}{\Delta_0}\right] \\ &= Y(\omega) + i\frac{X(\omega)}{\Delta_0}.\end{aligned} \tag{9}$$

Combining Eq. (7) and Eq. (9) shows that the Fourier transform is zero at $\omega = \Delta_0$. This effect is illustrated in Fig. 7. With the sigmoid basis, such pulses can be constructed straight-forwardly

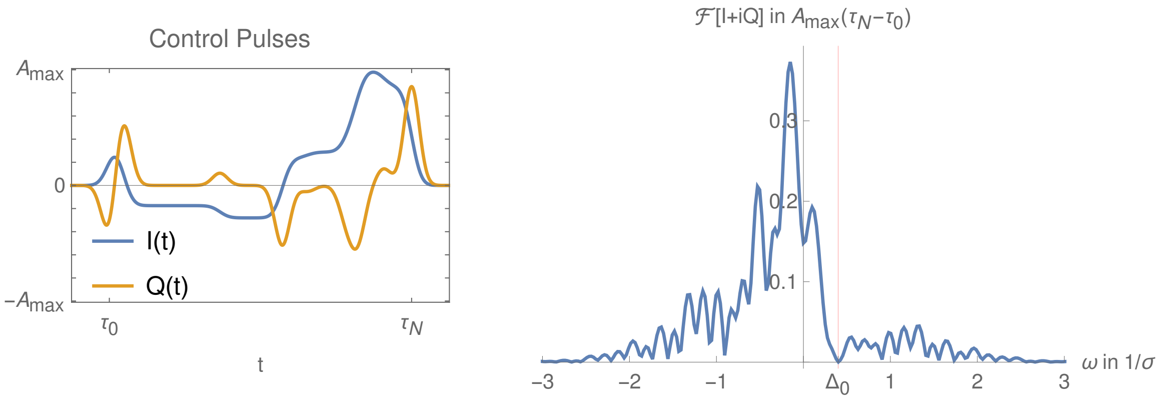


Figure 7: DRAG control pulse constructed with the sigmoid basis. (*left*) I- and Q-component calculated according to eq. (8) with a detuning of $\Delta_0$. (*right*) Pulse spectrum with a distinctive node at $\Delta_0$. This figure was taken from Ref [3] with the author's permission.

resulting in $I(t)$ being made up of sigmoids and $Q(t)$ of Gaussians, i.e. the sigmoids' derivatives. However, a similar approach could be applied to other bases too.

For completeness, it should be mentioned that higher orders of DRAG which include the relationship between the pulse amplitudes and detuning have not been discussed here, but could in principal also be included in such conditions.

---


[1] N. Khaneja, T. Reiss, C. Kehlet, T. Schulte-Herbrüggen, and S. J. Glaser, Optimal control of coupled spin dynamics: design of NMR pulse sequences by gradient ascent algorithms, Journal of Magnetic Resonance **172**, 296 (2005).

[2] A. I. Konnov and V. F. Krotov, On global methods for the successive improvement of control processes, Avtomatika i Telemekhanika **60**, 77 (1999).

[3] P. Rembold, *Quantum Optimal Control of Spin Systems and Trapped Atoms*, PhD thesis, Universität zu Köln and Università degli Studi di Padova (2022).

[4] F. Motzoi, J. M. Gambetta, P. Rebentrost, and F. K. Wilhelm, Simple Pulses for Elimination of Leakage in Weakly Nonlinear Qubits, Phys. Rev. Lett. **103**, 110501 (2009).

[5] C. C. Margossian, A review of automatic differentiation and its efficient implementation, WIREs Data Mining and Knowledge Discovery **9**, e1305 (2019), _eprint: https://onlinelibrary.wiley.com/doi/pdf/10.1002/widm.1305.

[6] N. Leung, M. Abdelhafez, J. Koch, and D. Schuster, Speedup for quantum optimal control from automatic differentiation based on graphics processing units, Physical Review A **95**, 042318 (2017).

[7] J. Bradbury, R. Frostig, P. Hawkins, M. J. Johnson, C. Leary, D. Maclaurin, G. Necula, A. Paszke, J. VanderPlas, S. Wanderman-Milne, and Q. Zhang, JAX: composable transformations of Python+NumPy programs (2018).

[8] D. P. Kingma and J. Ba, Adam: A Method for Stochastic Optimization (2017), arXiv:1412.6980 [cs].
